# Supplementary material for: OmniScientist: Toward a Co-evolving Ecosystem of Human and AI Scientists
Source: arXiv:2511.16931 source file (2025-12-14)
Supplement: Supplementary file 1 [file appendix.tex]

n% 各个赛道的模型列表说明

\begin{itemize}[leftmargin=3em]

    \item \textbf{Literature Review}: The current participants in this track include \textbf{OpenAI Deep Research}~\cite{openai_deep_research_2025}, \textbf{Sonar Deep Research} (Perplexity.ai)~\cite{perplexity_sonar_deep_research_2025}, \textbf{Qwen Deep Research}~\cite{qwen_deep_research_2025}, \textbf{Google/Gemini-2.5-pro}~\cite{google_gemini_2_5_pro_2025}, \textbf{MoonshotAI/Kimi-K2}~\cite{moonshotai_kimi_k2_2025}, \textbf{Anthropic/Claude-Opus-4.1}~\cite{anthropic_claude_opus_4_1_2025}, and our own \textbf{Astrum Deep Research}. 
    For the Deep Research models from OpenAI, Qwen, and Perplexity, we accessed them through their official APIs. In contrast, Gemini, Kimi, and Claude each provide Deep Research functionalities via their respective web platforms, but none currently offer public API access for Deep Research. Therefore, we employ each company’s flagship model to perform the Deep Research tasks, using the \texttt{OpenRouter} online-enabled versions for unified evaluation (by appending ``\texttt{:online}'' to the model name and configuring the \texttt{web\_search\_options} field in the request body).

    Since the interaction details of different Deep Research systems vary, some APIs prompt users to further clarify or refine their queries, while others do not. Such inconsistency may introduce bias in both user experience and evaluation when comparing models. To ensure fairness, we standardized the procedure by disabling query updates across all systems. Instead, we provided example prompts within the input box to help users articulate their research questions as clearly as possible in a single submission. In cases where an API requested additional clarification, we simply re-sent the user’s original input as the response. The amount of retrieved information, the presence of detailed citations, and the inclusion of reasoning traces were left to depend on each model’s intrinsic capabilities.

    \item \textbf{Ideation}:
    In this track, we primarily consider two agents: Deep Ideation and SciPIP~\cite{Wang2024SciPIPAL}. SciPIP constructs a dataset from a large corpus of AI-focused scientific papers, performing information extraction and retrieval for each publication. It subsequently generates research ideas by integrating document retrieval with model-based reasoning.

    \item \textbf{Hypothesis generation}: In this track, we consider two competing agents: MOOSE-Chem~\cite{Yang2024MOOSEChemLL} and SciMON~\cite{Wang2023SciMONSI}. MOOSE-Chem employs a multi-agent framework that leverages LLMs to perform retrieval and identification of hypotheses, generative extrapolation, and evaluation-based ranking. In contrast, SciMON retrieves ``inspiration'' from past scientific publications and explicitly refines idea proposals through iterative comparison with prior work until sufficient novelty is achieved. In addition to these two models, several other LLMs were included as participants for comparison: GPT-5, Gemini 2.5 Pro, Claude Sonnet 4.5, DeepSeek V3.2, Kimi K2, Qwen3 235B, and GLM 4.6.
    
    \item \textbf{Reviewer}: DeepReviewer~\cite{Weng2024CycleResearcherIA}

    \item \textbf{PaperQA}: For this track, PaperQA2~\cite{Skarlinski2024LanguageAA} serves as the primary candidate agent. It employs a toolset comprising ``Paper Search,'' ``Gather Evidence,'' ``Generate Answer,'' and ``Citation Traversal'' to enhance retrieval and response accuracy through a multi-step procedure.

    \item \textbf{Digital twin}: In this track, we primarily evaluate five agents: Second Me~\cite{Wei2025AInativeM2}, A-Mem Digital Twin~\cite{Xu2025AMEMAM}, MemoryOS Digital Twin~\cite{Kang2025MemoryOO}, HippoRAG Digital Twin~\cite{Gutierrez2024HippoRAGNI}, and Mem0 Digital Twin~\cite{Chhikara2025Mem0BP}.
    Second Me serves as the most directly comparable digital twin system. It is designed with an intelligent, persistent memory offloading architecture capable of retaining, organizing, and dynamically utilizing user-specific knowledge. By acting as an intermediary in user interactions, it automatically generates context-aware responses, pre-populates required information, and facilitates seamless communication with external systems, thereby significantly reducing cognitive load and interaction friction.
    A-Mem constructs an interconnected knowledge network through dynamic indexing and linking mechanisms, allowing newly incorporated memories to update the entire network in real time. MemoryOS introduces a three-tier hierarchical memory storage architecture and integrates four core functional modules—storage, update, retrieval, and generation—to dynamically capture and evolve user preferences. HippoRAG draws inspiration from the interaction between the hippocampus and neocortex in the human brain, constructing a hippocampus-like knowledge graph (KG) to achieve pattern separation and completion of knowledge. This design enables more efficient and faster online retrieval. Mem0 ensures coherence and consistency throughout extended dialogues by dynamically extracting, integrating, and retrieving key information from conversations.

\end{itemize}
